# Supplementary material for: Diagrammatic Exciton Basis Theory of the Photophysics of Pentacene Dimers
Source: arXiv:1707.04633 source file (2017-07-14)
Supplement: Supplementary file 1 [file Supporting_Info_BP0.pdf]

# Diagrammatic Exciton Basis Theory of the Photophysics of Pentacene Dimers

## Supporting Information

Souratosh Khan
*Department of Physics, University of Arizona Tucson, AZ 85721*

Sumit Mazumdar
*Department of Physics, University of Arizona*
*Department of Chemistry and Biochemistry, University of Arizona and*
*College of Optical Sciences, University of Arizona*
(Dated: July 14, 2017)

## I. TIPS-PENTACENE MONOMER - DETAILS OF MRSDCI CALCULATIONS

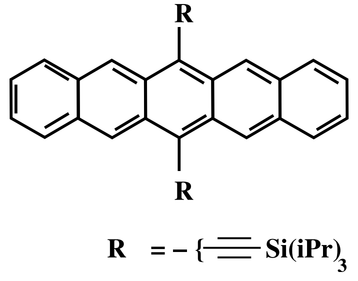


FIG. S1: TIPS-pentacene molecule

The presence of both center-of-inversion and mirror-plane symmetry means that the TIPS-pentacene molecule like its predecessor, pentacene, belongs to the $D_{2h}$ point group symmetry. As a consequence, the eigenstates belong to either of the following sub-groups: $A_g$, $B_{2u}$, $B_{3u}$ and $B_{1g}$. While the ground state has an $A_g$ symmetry, the lowest optical and triplet states both lie in the $B_{2u}$ subspace of their respective spin manifolds. Theoretical work on polyacenes have shown that the lowest absorption in the ground state absorption spectra is polarized along the short molecular axis[1]. In contrast, the lowest absorption in the triplet excited state absorption (ESA) spectra is polarized along the long molecular axis[2].

Given below are the computational methods (QCI - Quadruple Configuration Interaction where all single, double, triple and quadruple excitations from the HF ground state are included/MRSDCI) adopted, reference states ($N_{ref}$) and the dimension of the matrix diagonalized ($N_{total}$) in each of the sub-groups that allowed us to calculate the various absorption spectra for two different parameter sets.

TABLE S1: **U = 6.7 eV, $\kappa$ = 1.0**

| | $^1A_g$ | $^1B_{2u}$ | $^1B_{3u}$ | $^3A_g$ | $^3B_{2u}$ | $^3B_{1g}$ |
|---|---|---|---|---|---|---|
| Method | QCI | QCI | MRSDCI | MRSDCI | QCI | MRSDCI |
| $N_{ref}$ | 1 | 1 | 104 | 87 | 1 | 78 |
| $N_{total}$ | 1002823 | 1707547 | 346674 | 630871 | 3202443 | 512544 |

TABLE S2: **U = 7.7 eV, $\kappa$ = 1.3**

| | $^1A_g$ | $^1B_{2u}$ | $^1B_{3u}$ | $^3A_g$ | $^3B_{2u}$ | $^3B_{1g}$ |
|---|---|---|---|---|---|---|
| Method | QCI | QCI | MRSDCI | MRSDCI | QCI | MRSDCI |
| $N_{ref}$ | 1 | 1 | 86 | 72 | 1 | 94 |
| $N_{total}$ | 1002823 | 1707547 | 324326 | 721575 | 3202443 | 679048 |

## II. DETAILS OF MRSDCI CALCULATIONS FOR BPn

### I. Ground state absorption : $S_0 \rightarrow S_1$

We employ the MRSDCI method to calculate the energy and wavefunctions of the dipole allowed states in the singlet subspace, namely $S_1$ and $S_2$. As discussed in the main text, we retain 24 active HF MO orbitals (20 localized on the 2 TIPS-Pentacene molecules in BP0 and BP1; 4 localized on benzene in BP1) from the available space. We then proceed to calculate the matrix elements $\langle S_0|\mu|S_1\rangle$ and $\langle S_0|\mu|S_1\rangle$ where $\mu = e\sum \vec{r_i} n_i$ . The Table below shows the reference states ($N_{ref}$) and the dimension of the Hamiltonian matrix ($N_{total}$) used in computing the energies of $S_1$ and $S_2$. The process of updating $N_{ref}$ and $N_{total}$ is carried out till a desired convergence of the relevant optical states (Inclusion of all configurations in $N_{ref}$ whose normalized coefficients is $\geq 0.04$.) is achieved. The absorption spectrum, $\alpha(\omega)$ is given by the following expression.

$$\alpha(\omega) = \sum_{i,j} \frac{\omega[(\mu^x_{i,j})^2 + (\mu^y_{i,j})^2 + (\mu^z_{i,j})^2]\delta}{[(\omega - \omega_j + \omega_i)^2 + \delta^2]} \tag{1}$$

Here, $i$ and $j$ are the initial and final states respectively.

No. of Active Orbitals : 24

| | BP0 | | | | BP1 | | | |
|---|---|---|---|---|---|---|---|---|
| | $\theta = 0$ | $\theta = 30$ | $\theta = 45$ | $\theta = 60$ | $\theta = 0$ | $\theta = 30$ | $\theta = 45$ | $\theta = 60$ |
| $N_{ref}$ | 161 | 157 | 157 | 145 | 177 | 193 | 155 | 152 |
| $N_{total}$ | 2317162 | 2379524 | 2431684 | 2427576 | 2206000 | 2800266 | 2251134 | 2455660 |

## II. SCI result

The linear absorption spectra for TPc, BP0 and BP1 were also computed in the SCI (Singles Configuration Interaction) limit where only 1e-1h excitations from the HF ground state were retained. Interestingly, we observe that the lower energy absorption in dimers is slightly red-shifted. This is because of the inclusion of all possible single excitations and the retention of the entire active space of HF MOs in the calculation.

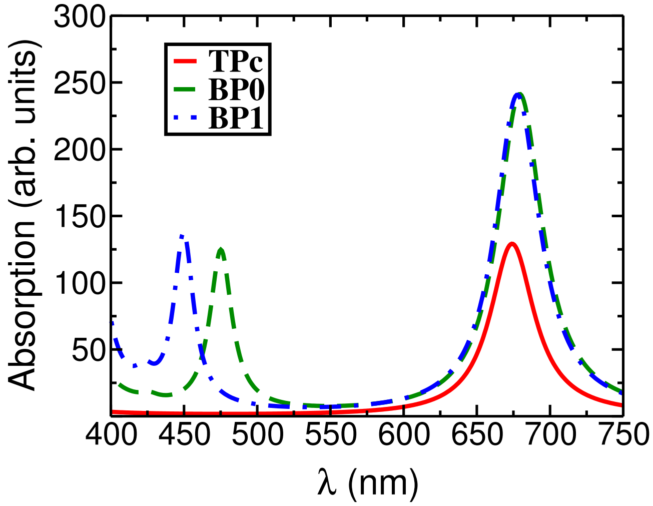


FIG. S2: Calculated linear absorption spectrum (SCI) for TIPS monomer, BP0 and BP1 ($U = 6.7$ eV, $\kappa = 1.0$).

## III. ESA CALCULATIONS

We follow the same procedure as has been outlined in the previous section for calculating Excited State Absorption (ESA) spectra from the singlet, triplet and triplet-triplet excitons. The initial target state from which absorption is to be calculated is identified and the relevant dipole allowed states are determined by an iterative process of updating $N_{ref}$ and $N_{total}$.

### I. Calculation of singlet ESA

The singlet ESA has strong optical signatures both in the infra-red (IR) and visible (VIS) regions. The ESA spectrum along with the computational details of the MRSDCI calculation for calculating it are presented below. In this section, we have only shown the wavefunctions of the final states in the VIS region ($\sim$ 650 nm). The origin of the peaks at $\sim$ 2200 nm ($S_1^a$), 1800 nm ($S_1^b$) and 1200 nm ($S_1^c$) has been described in the main text. In the visible spectrum, it is clear from the wavefunctions in Fig. S3(b) that the final states are primarily composed of 2e-2h excitations (CT and intramolecular) and is therefore a signature of dimer absorption.

No. of Active Orbitals : 24

| | U = 6.7 eV, $\kappa$ = 1.0 |
|---|---|
| $N_{ref}$ | 260 |
| $N_{total}$ | 3560877 |

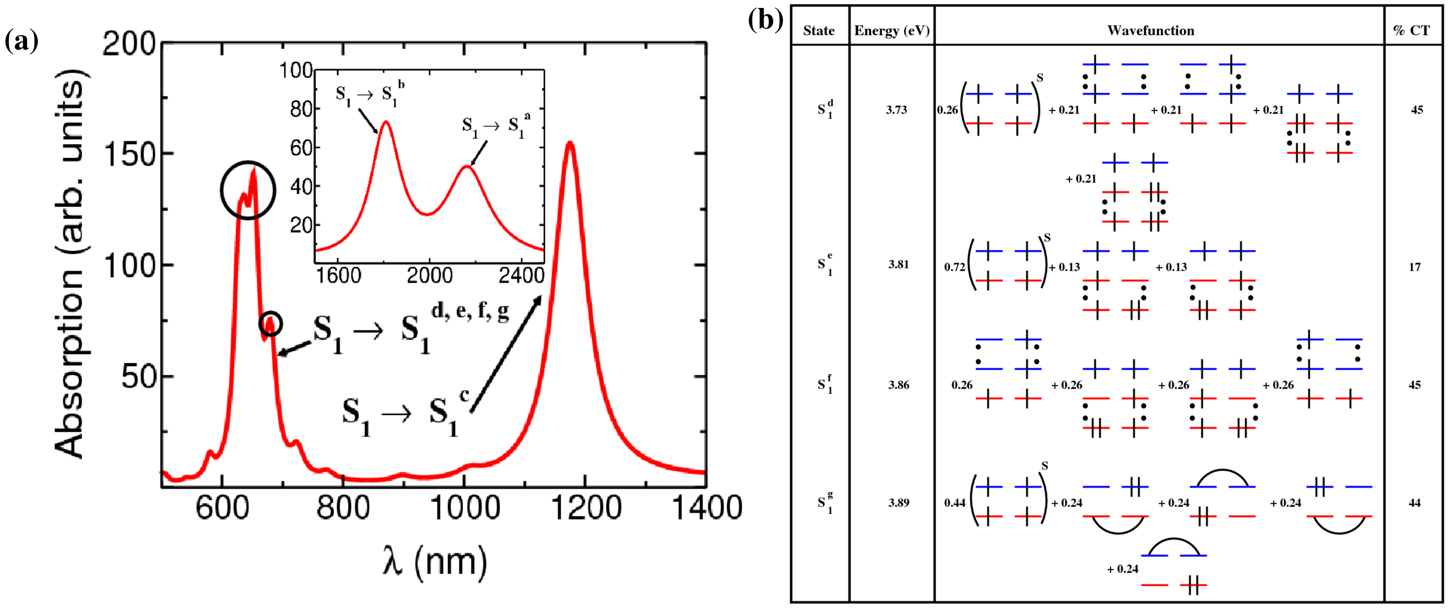


FIG. S3: (a) Singlet ESA spectrum in the mid IR, near IR and VIS regions. (b) Final states that contribute to a strong absorption in the VIS region of the ESA spectra with their dominant contributions, energies and degree of CT character. To distinguish the 2e-2h excitation that involves HOMO → LUMO transitions within each pentacene molecule in BP0 from the $^1(TT)_1$ state, it has been included within parenthesis along with a superscript 'S'. Transitions to singlet states that involve MOs far away from the chemical potential are depicted by diagrams that include dots above/below the LUMO/HOMO levels.

## II. Calculation of triplet ESA

### 1. $E(T_1)$

The energies of the lowest triplet state ($T_1$) and the dipole allowed states ($T_N$) are determined by retaining 20 active MOs. We have presented Tables below of our calculated E($T_1$) as well as the $N_{ref}$ and $N_{total}$ in BP0 and BP1. The dimension of the Hamiltonian in the triplet subspace is much larger than the one in the singlet subspace for the same number of excited states. This limits us from using higher HF MOs in our CI calculation. However, with 20 active MOs, the size of the basis space still exceeds a million and hence our calculations would include the most dominant higher order configurations in the description of the eigenstates.

| | BP0, $\theta = 0$ | | BP1, $\theta = 0$ | |
|---|---|---|---|---|
| | U = 6.7 eV, $\kappa$ = 1.0 | U = 7.7 eV, $\kappa$ = 1.3 | U = 6.7 eV, $\kappa$ = 1.0 | U = 7.7 eV, $\kappa$ = 1.3 |
| E($T_1$) | 0.98 eV | 0.9 eV | 1.03 eV | 0.96 eV |

### *2. Triplet ESA* : $\boldsymbol{T}_1 \rightarrow \boldsymbol{T}_N$

| | BP0, $\theta = 0$ | | BP1, $\theta = 0$ | |
|---|---|---|---|---|
| | U = 6.7 eV, $\kappa$ = 1.0 | U = 7.7 eV, $\kappa$ = 1.3 | U = 6.7 eV, $\kappa$ = 1.0 | U = 7.7 eV, $\kappa$ = 1.3 |
| $N_{ref}$ | 71 | 103 | 96 | 120 |
| $N_{total}$ | 1465715 | 1877853 | 1725338 | 2471792 |

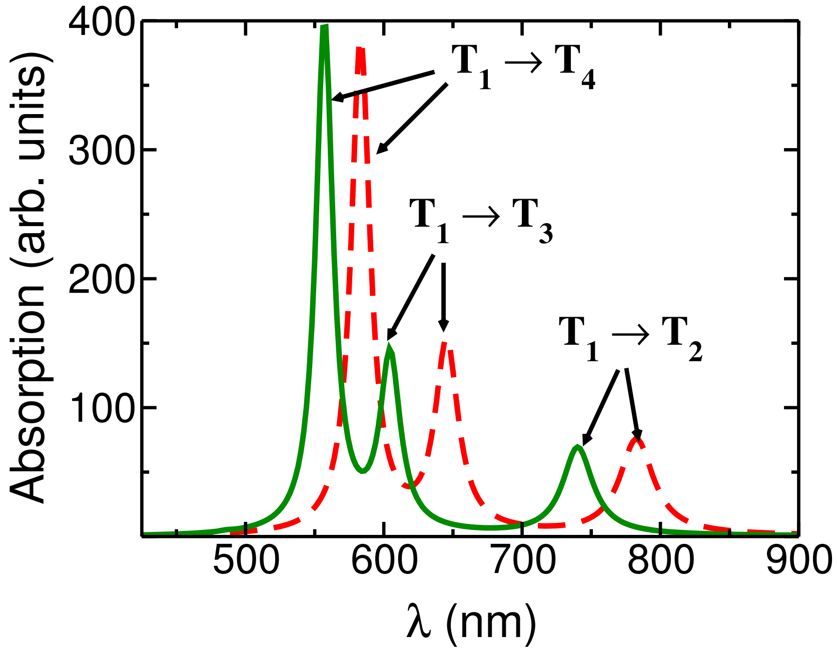


FIG. S4: BP0 - Triplet ESA for U = 6.7 eV, $\kappa$ = 1.0 (dashed red) and U = 7.7 eV, $\kappa$ = 1.3 (solid green) and $\theta = 0°$.

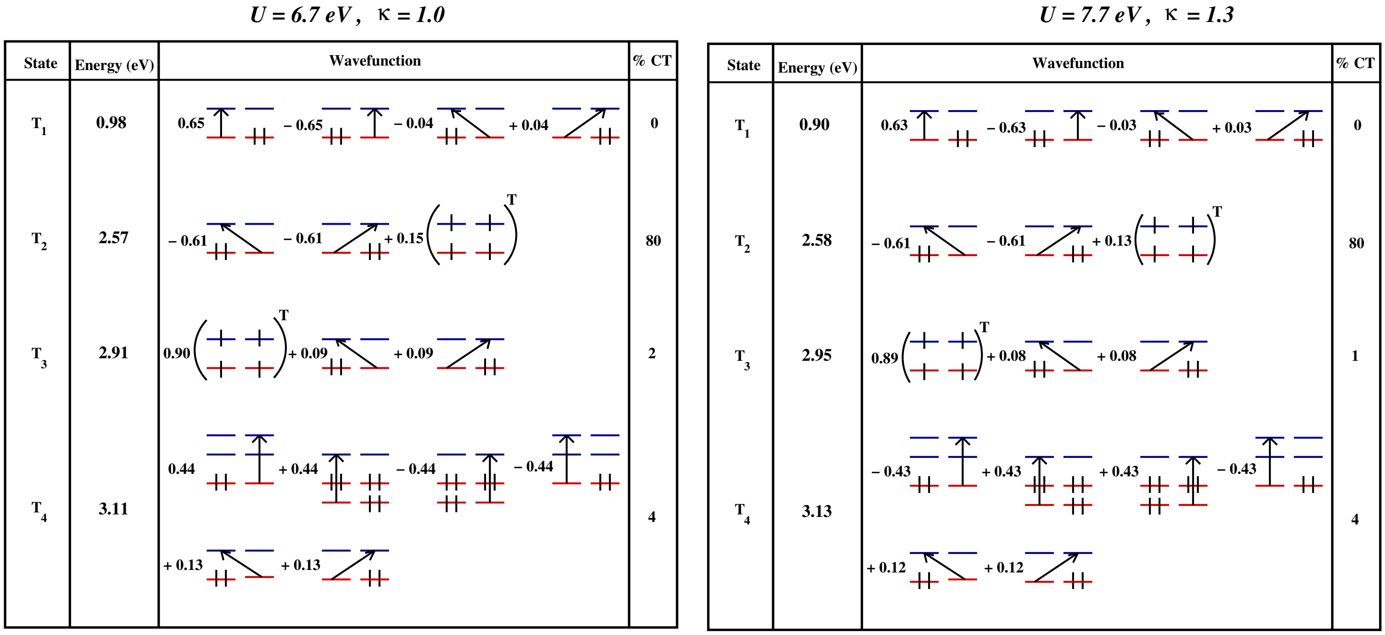


FIG. S5: Wavefunctions, energies and degree of CT character of $T_1$, $T_2$, $T_3$, $T_4$ in BP0 with $\theta = 0°$. The arrows represent triplet excitations between the respective molecular orbitals, given by the expression : $\frac{1}{\sqrt{3}}[a^{\dagger}_{i,\uparrow}a_{j,\downarrow} + a^{\dagger}_{i,\downarrow}a_{j,\uparrow} + \frac{1}{\sqrt{2}}(a^{\dagger}_{i,\uparrow}a_{j,\uparrow} + a^{\dagger}_{i,\downarrow}a_{j,\downarrow})]|G\rangle$. Neither the dominant contributions to the wavefunctions nor their relative weights change significantly between the two parameter sets.

## III. $^1$(TT)$_1$ state and Triplet-Triplet ESA : $^1$(TT)$_1$ → $^1$(TT)$_N$

The triplet-triplet ESA spectra are evaluated for BP0 and BP1 with 24 Active MOs respectively. In reality, even this would be insufficient for obtaining the spectrum in BP1 due to an increase in the energy of the CT states from an inadequate number of HF MOs. At the same time, it becomes computationally expensive to perform a high-order CI calculation with such a large basis space. We only present here the triplet-triplet ESA spectra for BP0 and compute the transition dipole moments from the $^1$(TT)$_1$ state in BP1 to all the relevant states in the far and mid IR region only.

| | BP0, $\theta = 0$ | | BP1, $\theta = 0$ | |
|---|---|---|---|---|
| | U = 6.7 eV, $\kappa = 1.0$ | U = 7.7 eV, $\kappa = 1.3$ | U = 6.7 eV, $\kappa = 1.0$ | U = 7.7 eV, $\kappa = 1.3$ |
| $N_{ref}$ | 145 | 103 | 169 | 160 |
| $N_{total}$ | 2130960 | 1973776 | 2178900 | 2171638 |

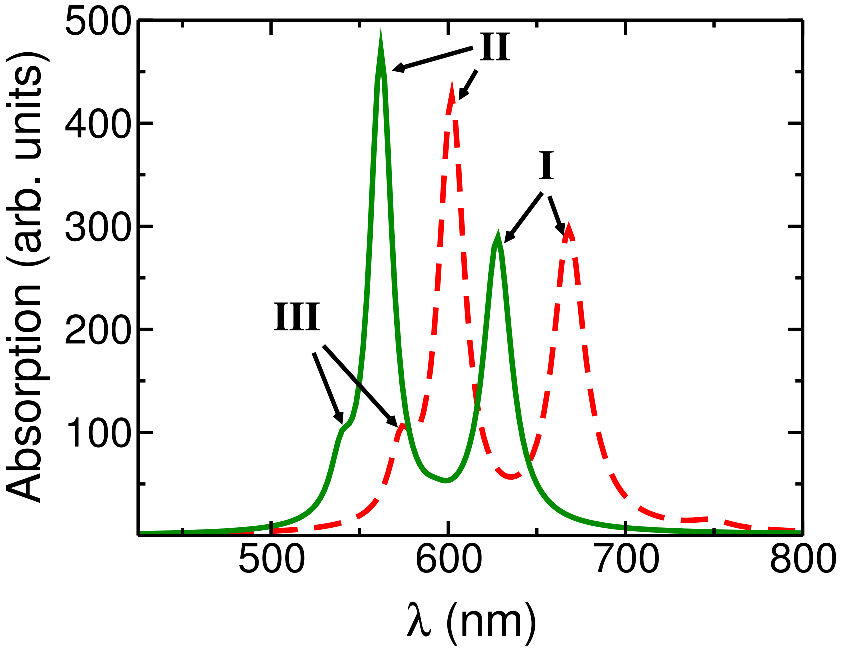


FIG. S6: Triplet-Triplet ESA spectra for U = 6.7 eV, $\kappa$ = 1.0 (dashed red) and U = 7.7 eV, $\kappa$ = 1.3 (solid green). I : $^1(TT)_1 \rightarrow {}^1(TT)_2$; II : $^1(TT)_1 \rightarrow {}^1(TT)_3$; III : $^1(TT)_1 \rightarrow {}^1(TT)_4$

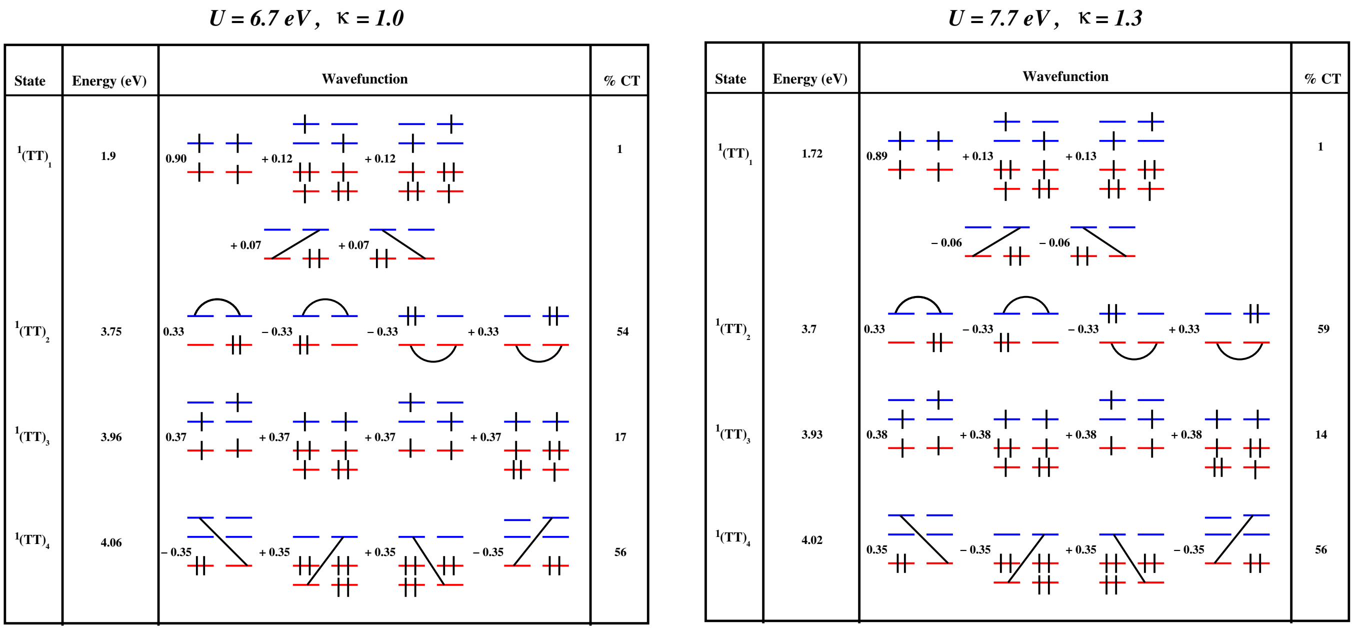


FIG. S7: Wavefunctions, energies and degree of CT character of $^1(TT)_1$, $^1(TT)_2$, $^1(TT)_3$, $^1(TT)_4$ states of BP0.

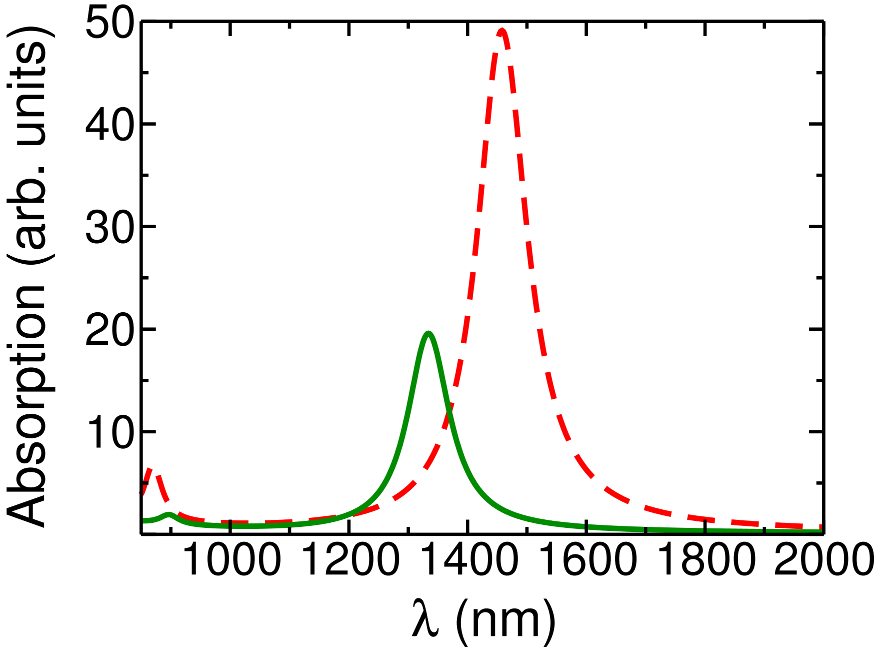


FIG. S8: Comparsion of the triplet-triplet spectra in BP0 (dashed red) and BP1 (solid green) in the mid-IR region. Our theoretical result is in accordance with the unpublished results from reference 3, i.e. the absorption in mid-IR becomes weaker with the addition of phenyl linkers.

[1] Priya Sony and Alok Shukla. Large-scale correlated calculations of linear optical absorption and low-lying excited states of polyacenes: Pariser-Parr-Pople hamiltonian. *Phys. Rev. B*, 75:155208, Apr 2007.
[2] H. Chakraborty and A. Shukla. Theory of triplet optical absorption in oligoacenes: From naphthalene to heptacene. *J. Chem. Phys.*, 141:164301, 2014.
[3] M. Sfeir. private communication.
